# Supplementary material for: SSD: A Unified Framework for Self-Supervised Outlier Detection
Source: arXiv:2103.12051 source file (2021-03-22)
Supplement: Supplementary file 2 [file appendix.tex]

We cluster representations learned with SimCLR on CIFAR-10 with kmeans using 100 clusters. We show a subset of images from the tightest and loosest cluster in following figure. 

\begin{figure}
     \centering
     \begin{subfigure}[b]{0.49\textwidth}
         \centering
         \includegraphics[width=\textwidth]{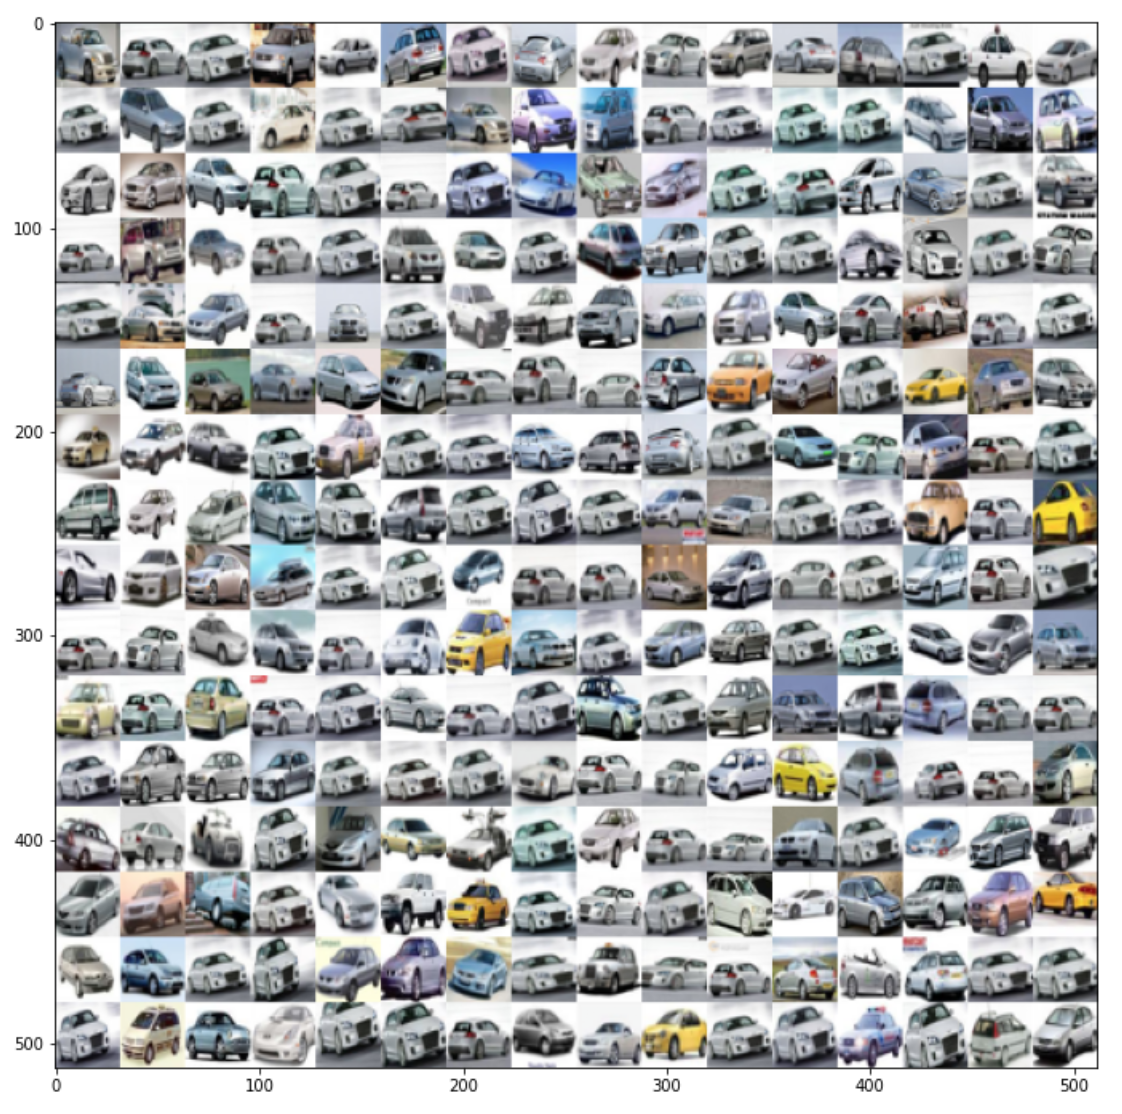}
         \caption{Cluster where most examples are closest to the centroid.}
     \end{subfigure}
     \hfill
     \begin{subfigure}[b]{0.49\textwidth}
         \centering
         \includegraphics[width=\textwidth]{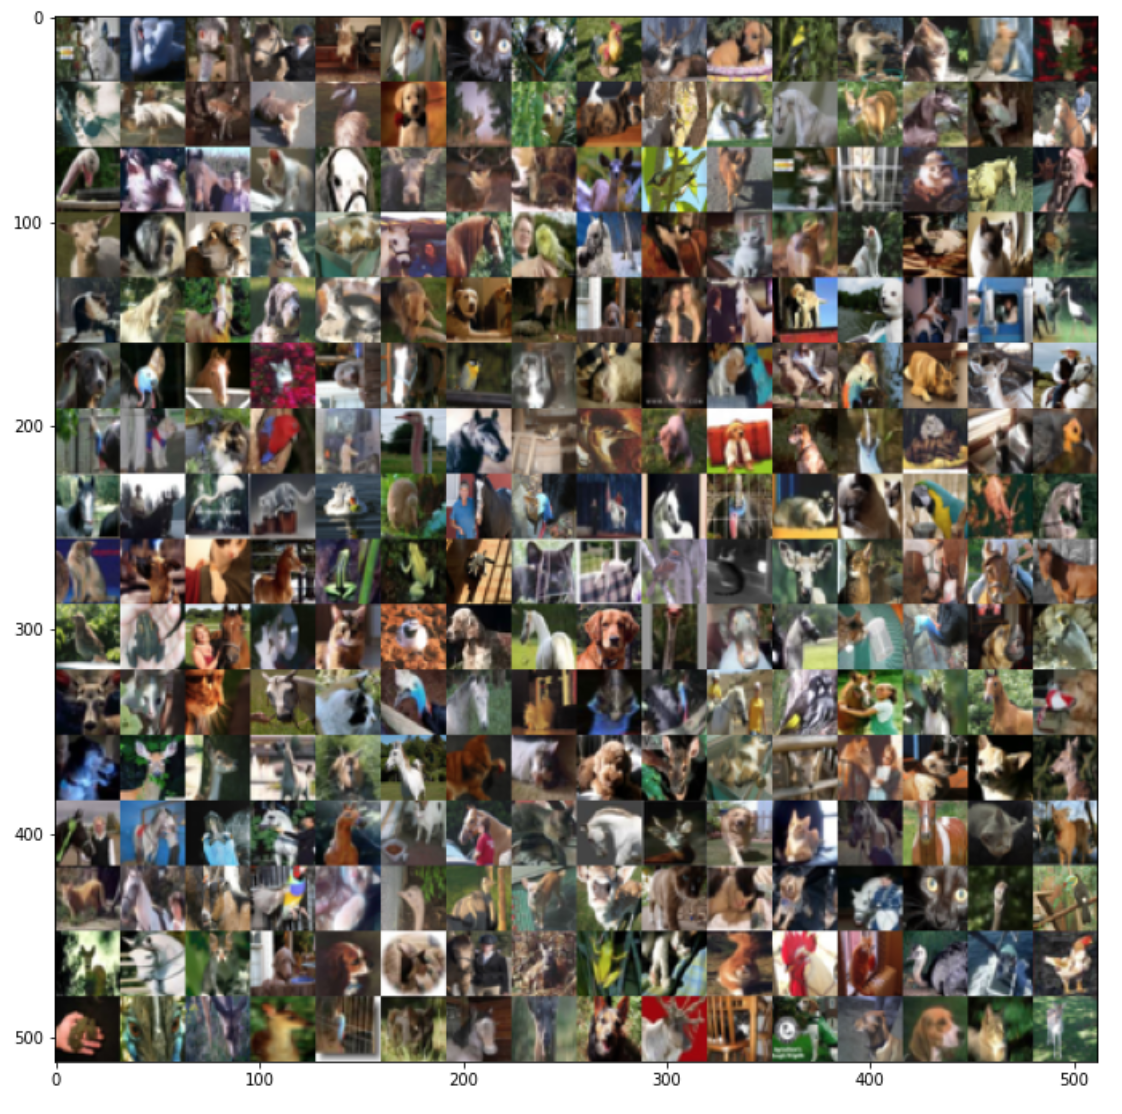}
         \caption{Cluster where most examples are farthest to the centroid.}
     \end{subfigure}
    
    \caption{Two extremes of the clusters, tightest and loosest, obtained with Self-supervised training. Use entropy to characterize these clusters.}
\end{figure}



\section{Notes}
\begin{itemize}
    \item Note that instead of entropy, a baseline approach, is to crate histogram of distances from cluster centroid. Both Mahalanobis and the Contra-detector roughly use this technique. We can show that with this is not effective as entropy is able to discriminate better. Additionally it can also be used with supervised-detectors to improve their performance.
    \item With supervised networks, we have to see which technique helped more: Cluster, instead of class conditional, modelling or the use of entropy instead of distances. 
    \item Pitch: We should pitch our algorithm on using multiple cluster distances as a phenomenon, as it is also application in multiple detectors. Something which shows that OOD data fall close to multiple clusters simultaneously and should be considered. We can then pitch the approach of using entropy to measure it. Something like thick boundary, uniform distribution etc.
\end{itemize}


\noindent \textbf{Outlier detection. } Here we provide a concise review of outlier detection literature.
\begin{itemize}
    \item Use in communication, financial frauds, fake news, heath-care, security etc.
    \item Global outliers: Deviates significantly from the data itself. We do have results saying that simply assuming having a Gaussian prior on in-distribution, we can detector more than half of the OOD images. We can start with this experiment showing that \textit{most of OOD points are global outliers}, which can be easily detected. 
    \item 
\end{itemize}



\newpage

\section{TRASH}

\begin{table}[!htb]
\centering
\caption{ONLY WHEN THRESHOLDING IS DONE WITH TRAIN DATA. Comparison of our approach with state of the art detectors. Note that we are still using a sub-optimal setup (ResNet18 network, no hyperparameter tuning etc), as the goal was to get some quick numbers. Our method's performance is expected to improve further as we dig deeper. Note that all of these required labelled training data, and some even need OOD data for calibration, or pre-training on ImageNet. Our approach have none of these requirements and only require a set of unlabelled in-distribution images. We already achieve state-of-the-art FPR on CIFAR-10. Also CIFAR100 as OOD is hardest to detect, signalling that out methods performs best when the detection is hardest, a crucial innovation in OOD detection.}
\resizebox{0.95\textwidth}{!}{
\begin{tabular}{ccc|cc|cc}
\toprule
 & \multicolumn{2}{c}{CIFAR100} & \multicolumn{2}{c}{SVHN} & \multicolumn{2}{c}{\begin{tabular}[c]{@{}c@{}}Gaussian \\ Noise\end{tabular}} \\  \cmidrule{2-3} \cmidrule{4-5} \cmidrule{6-7}
 & FPR (TPR=95)     & AUROC     & FPR (TPR=95)   & AUROC   & FPR (TPR=95)                              & AUROC  \\ \midrule
Softmax probability~\citep{hendrycks2016baseline} & -    & 86.4 & -   & 89.9 & -   & -     \\
ODIN~\cite{liang2017odin}          & -    & 85.8 & -   & 96.7 & -   & -     \\
Mahalanobis distance~\citep{lee2018unifiedOOD}    & -    & 88.2 & -   & 99.1 & -   & -     \\
Residual flows~\citep{zisselman2020resflow} & -    & 89.4 & -   & 99.1 & -   & -     \\
\textbf{Ours (100 clusters)}  & \textbf{28.5} & 90.6 & 9.1 & 96.9 & 2.0 & 99.0  \\
\textbf{Ours (500 clusters)}  & \textbf{20.3} & 92.4 & 5.6 & 97.2 & - & -  \\
\textbf{Ours (2000 clusters)}  & \textbf{16.9} & \textbf{93.1} & 5.6 & 97.3 & - & -  \\
\textbf{Ours (10 clusters) + with labels}  & 22.1 & 91.3 & 9.3 & 97.3 & 3.1 & 99.1  \\
\textbf{Ours (100 clusters) + with labels}  & 39.6 & 81.2 & 21.9 & 90.7 & 9.3 & 95.9  \\
Sup + Rotation-SSL~\citep{hendrycks2019SSLOOD} & -    & 90.9 & -   & 98.9 & -   & -     \\
Sup + SimCLR-SSL~\citep{Winkens2020ContrastiveOOD} (SOTA)  & 39.9 & 92.9 & \textbf{2.8} & \textbf{99.5} & 0.3 & 100.0 \\\bottomrule
\end{tabular}}
\end{table}


\begin{table}[!htb]
\centering
\caption{ONLY WHEN THRESHOLDING IS DONE WITH TRAIN DATA. Using CIFAR100 as in-distribution, with ResNet18 network.}
\resizebox{0.95\textwidth}{!}{
\begin{tabular}{ccc|cc|cc}
\toprule
 & \multicolumn{2}{c}{CIFAR100} & \multicolumn{2}{c}{SVHN} & \multicolumn{2}{c}{\begin{tabular}[c]{@{}c@{}}Gaussian \\ Noise\end{tabular}} \\  \cmidrule{2-3} \cmidrule{4-5} \cmidrule{6-7}
 & FPR (TPR=95)     & AUROC     & FPR (TPR=95)   & AUROC   & FPR (TPR=95)                              & AUROC  \\ \midrule
\textbf{Ours (100 clusters)}  & 59.7 & 84.8 & 19.8 & 94.1 & 3.0 & 99.1  \\
\textbf{Ours (500 clusters)}  & \textbf{40.5} & \textbf{89.7} & \textbf{11.7} & \textbf{95.7} & 1.8 & 99.1 \\
Sup + SimCLR-SSL~\citep{Winkens2020ContrastiveOOD} (SOTA)  &  81.8 & 78.3 & 23.3 & 95.6 & \textbf{0.2} & \textbf{99.9} \\ \bottomrule
\end{tabular}}
\end{table}
